# Supplementary material for: Semi-supervised Quality Evaluation of Colonoscopy Procedures
Source: arXiv:2305.10090 source file (2023-05-17)
Supplement: Supplementary file 1 [file sm.tex]

\documentclass[runningheads]{llncs}

\usepackage[T1]{fontenc}

\title{Semi-supervised Quality Evaluation of \\ Colonoscopy Procedures}
%{Unsupervised Metrics for Assessing Colonoscopy Quality}
\author{}
\institute{Supplementary Material, ID 958}
% \date{October 2022}

\usepackage[square,sort,comma,numbers]{natbib}
\usepackage{graphicx}
\usepackage{pgfplots}
\usepackage{pgfplotstable}
\usepackage[export]{adjustbox}[2011/08/13]
\usepackage{dsfont}
\usepackage{mathtools}
\usepackage{caption}
\usepackage{subcaption}

\begin{document}

\maketitle

\begin{figure}
\centering
\captionsetup[subfigure]{labelformat=empty,justification=centering,aboveskip=1pt,belowskip=1pt}
    \begin{tabular}[c]{c c c c c c c c c c c}
    
    \centering
    
    \begin{subfigure}[t]{0.115\textwidth}
    \centering
    \caption*{Cluster}
    \end{subfigure}
    
    \begin{subfigure}[t]{0.081\textwidth}
    \centering
    \caption*{\#0}
    \end{subfigure}
    
    &
    
    \begin{subfigure}[t]{0.081\textwidth}
    \centering
    \caption*{\#1}
    \end{subfigure}
    
    &
    
    \begin{subfigure}[t]{0.081\textwidth}
    \centering
    \caption*{\#2}
    \end{subfigure}
    
    &
    
    \begin{subfigure}[t]{0.081\textwidth}
    \centering
    \caption*{\#3}
    \end{subfigure}
    
    &
    
    \begin{subfigure}[t]{0.081\textwidth}
    \centering
    \caption*{\#4}
    \end{subfigure}
    
    &
    
    \begin{subfigure}[t]{0.081\textwidth}
    \centering
    \caption*{\#5}
    \end{subfigure}
    
    &
    
    \begin{subfigure}[t]{0.081\textwidth}
    \centering
    \caption*{\#6}
    \end{subfigure}
    
    &
    
    \begin{subfigure}[t]{0.081\textwidth}
    \centering
    \caption*{\#7}
    \end{subfigure}
    
    &
    
    \begin{subfigure}[t]{0.081\textwidth}
    \centering
    \caption*{\#8}
    \end{subfigure}
    
    &
    
    \begin{subfigure}[t]{0.081\textwidth}
    \centering
    \caption*{\#9}
    \end{subfigure}
    
    \\

    \begin{subfigure}[t]{0.115\textwidth}
    \centering
    \vspace{1.9cm}
    Samples
    \end{subfigure}
    
    \begin{subfigure}[t]{0.081\textwidth}
    \centering
    \includegraphics[width=1\linewidth]{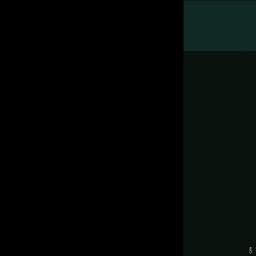}
    \includegraphics[width=1\linewidth]{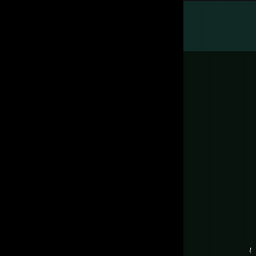}
    \includegraphics[width=1\linewidth]{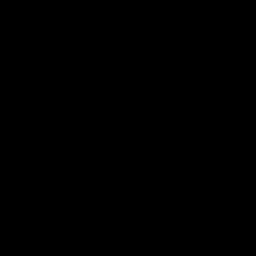}
    \includegraphics[width=1\linewidth]{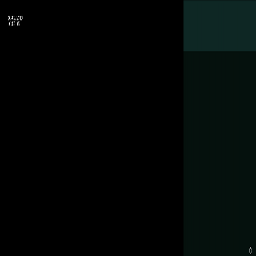}
    \includegraphics[width=1\linewidth]{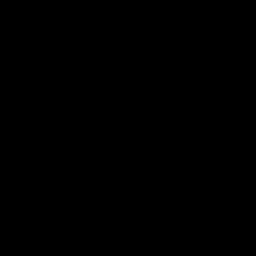}
    \includegraphics[width=1\linewidth]{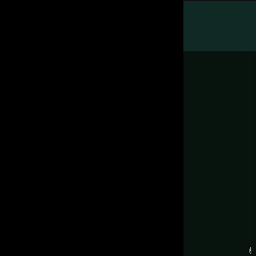}
    \end{subfigure}
    
    &
    
    \begin{subfigure}[t]{0.081\textwidth}
    \centering
    \includegraphics[width=1\linewidth]{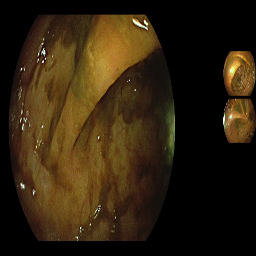}
    \includegraphics[width=1\linewidth]{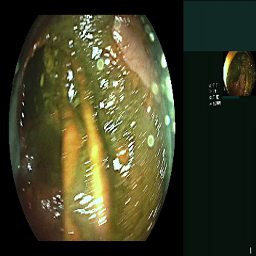}
    \includegraphics[width=1\linewidth]{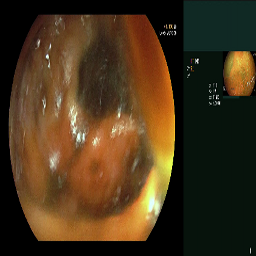}
    \includegraphics[width=1\linewidth]{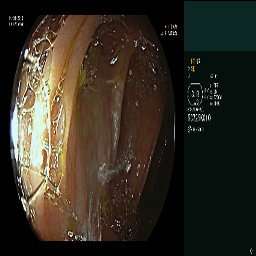}
    \includegraphics[width=1\linewidth]{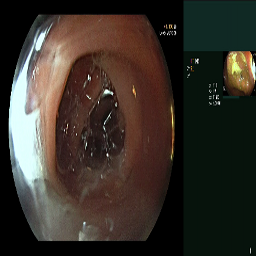}
    \includegraphics[width=1\linewidth]{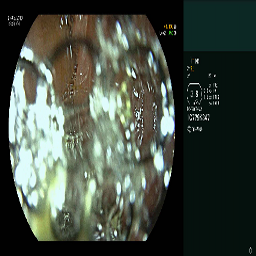}
    \end{subfigure}
    
    &
    
    \begin{subfigure}[t]{0.081\textwidth}
    \centering
    \includegraphics[width=1\linewidth]{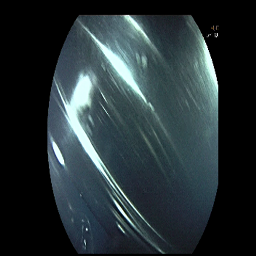}
    \includegraphics[width=1\linewidth]{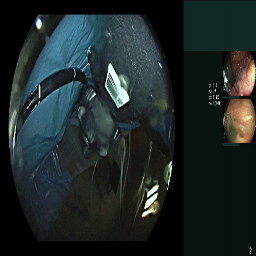}
    \includegraphics[width=1\linewidth]{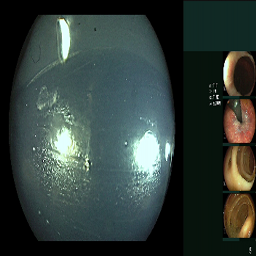}
    \includegraphics[width=1\linewidth]{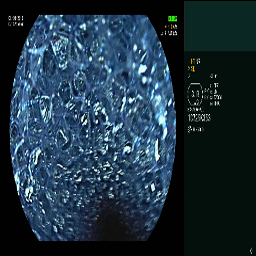}
    \includegraphics[width=1\linewidth]{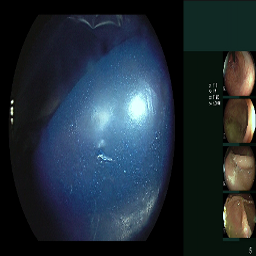}
    \includegraphics[width=1\linewidth]{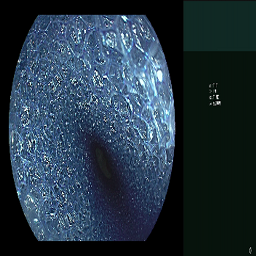}
    \end{subfigure}
    
    &
    
    \begin{subfigure}[t]{0.081\textwidth}
    \centering
    \includegraphics[width=1\linewidth]{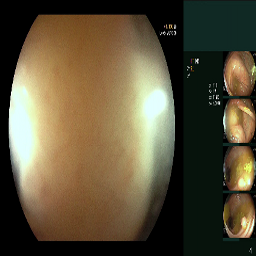}
    \includegraphics[width=1\linewidth]{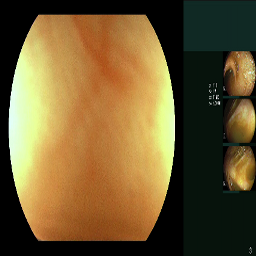}
    \includegraphics[width=1\linewidth]{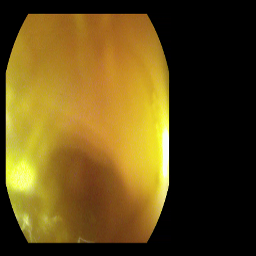}
    \includegraphics[width=1\linewidth]{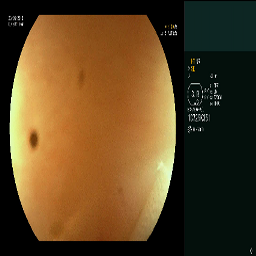}
    \includegraphics[width=1\linewidth]{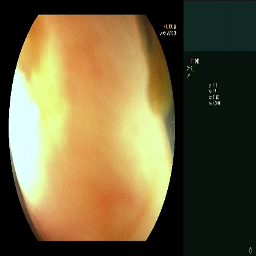}
    \includegraphics[width=1\linewidth]{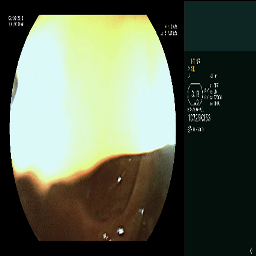}
    \end{subfigure}
    
    &
    
    \begin{subfigure}[t]{0.081\textwidth}
    \centering
    \includegraphics[width=1\linewidth]{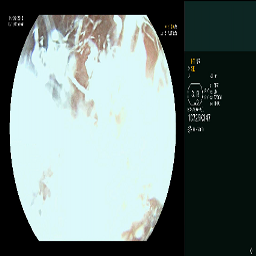}
    \includegraphics[width=1\linewidth]{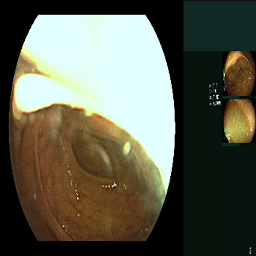}
    \includegraphics[width=1\linewidth]{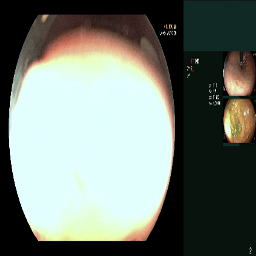}
    \includegraphics[width=1\linewidth]{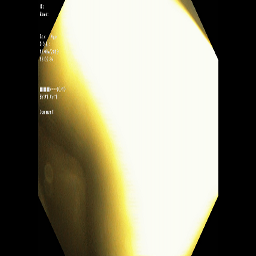}
    \includegraphics[width=1\linewidth]{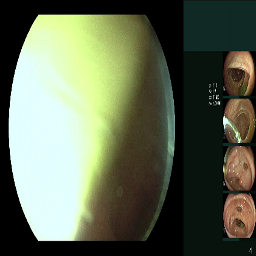}
    \includegraphics[width=1\linewidth]{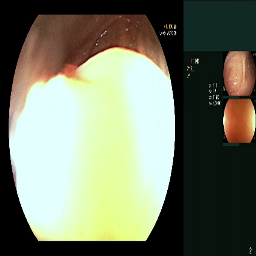}
    
    \end{subfigure}
    
    &
    
    \begin{subfigure}[t]{0.081\textwidth}
    \centering
    \includegraphics[width=1\linewidth]{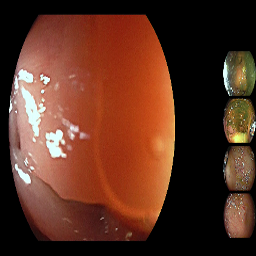}
    \includegraphics[width=1\linewidth]{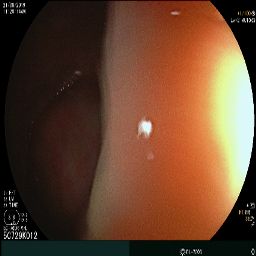}
    \includegraphics[width=1\linewidth]{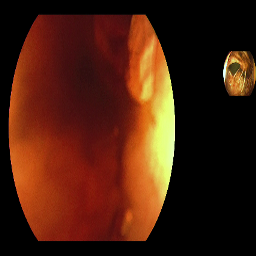}
    \includegraphics[width=1\linewidth]{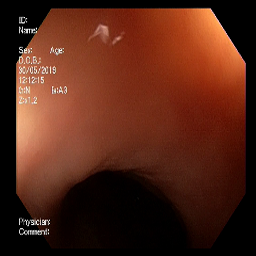}
    \includegraphics[width=1\linewidth]{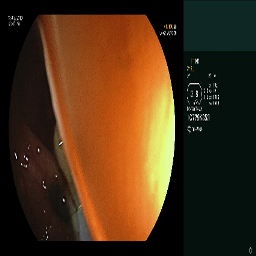}
    \includegraphics[width=1\linewidth]{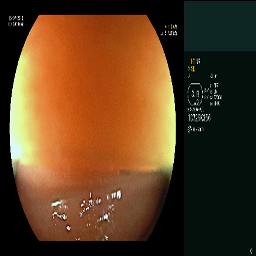}
    \end{subfigure}
    
    &
    
    \begin{subfigure}[t]{0.081\textwidth}
    \centering
    \includegraphics[width=1\linewidth]{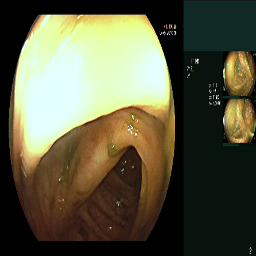}
    \includegraphics[width=1\linewidth]{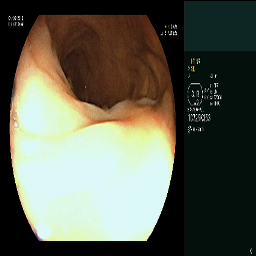}
    \includegraphics[width=1\linewidth]{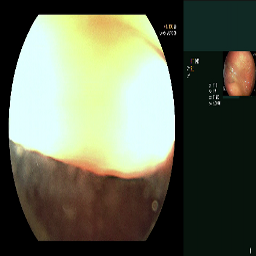}
    \includegraphics[width=1\linewidth]{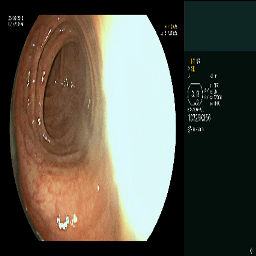}
    \includegraphics[width=1\linewidth]{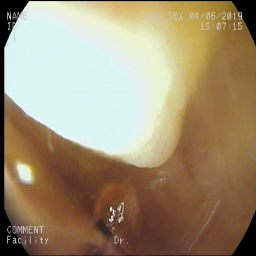}
    \includegraphics[width=1\linewidth]{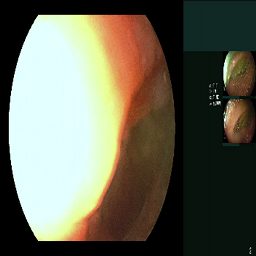}
    \end{subfigure}
    
    &
    
    \begin{subfigure}[t]{0.081\textwidth}
    \centering
    \includegraphics[width=1\linewidth]{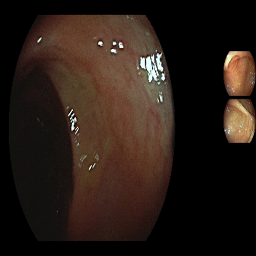}
    \includegraphics[width=1\linewidth]{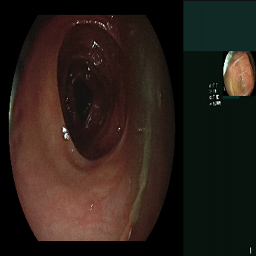}
    \includegraphics[width=1\linewidth]{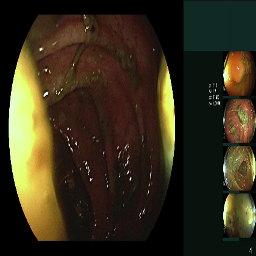}
    \includegraphics[width=1\linewidth]{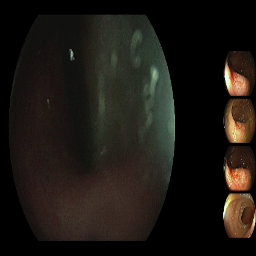}
    \includegraphics[width=1\linewidth]{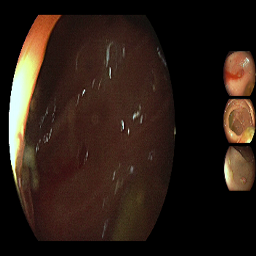}
    \includegraphics[width=1\linewidth]{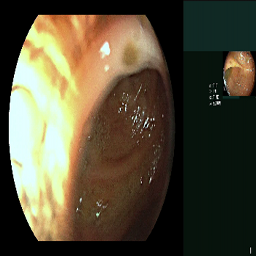}
    \end{subfigure}
    
    &
    
    \begin{subfigure}[t]{0.081\textwidth}
    \centering
    \includegraphics[width=1\linewidth]{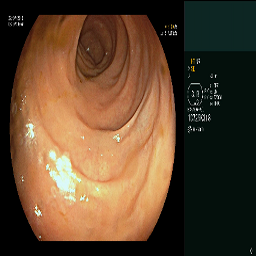}
    \includegraphics[width=1\linewidth]{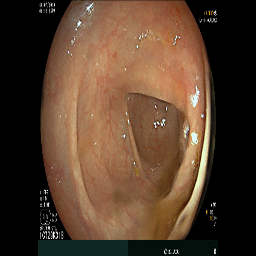}
    \includegraphics[width=1\linewidth]{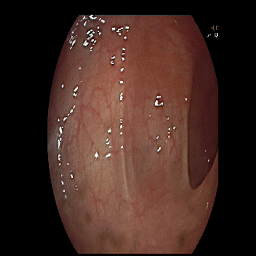}
    \includegraphics[width=1\linewidth]{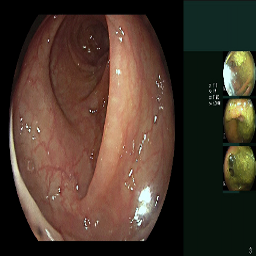}
    \includegraphics[width=1\linewidth]{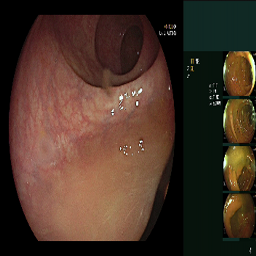}
    \includegraphics[width=1\linewidth]{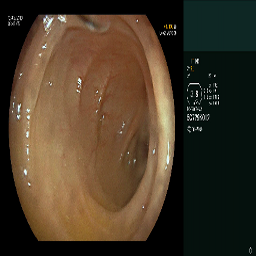}
    \end{subfigure}
    
    &
    
    \begin{subfigure}[t]{0.081\textwidth}
    \centering
    \includegraphics[width=1\linewidth]{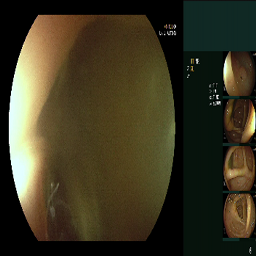}
    \includegraphics[width=1\linewidth]{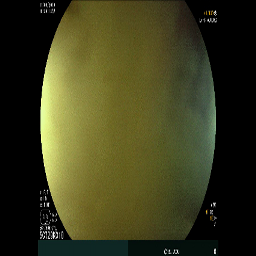}
    \includegraphics[width=1\linewidth]{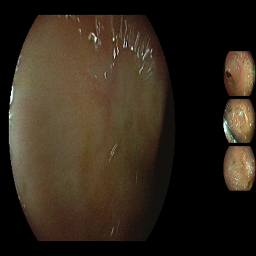}
    \includegraphics[width=1\linewidth]{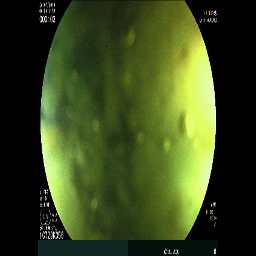}
    \includegraphics[width=1\linewidth]{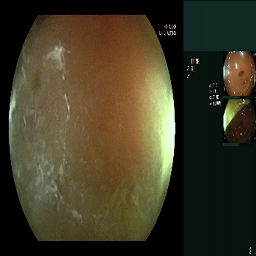}
    \includegraphics[width=1\linewidth]{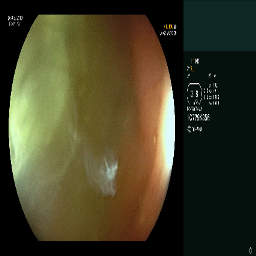}
    \end{subfigure}
    
    \\
        %array([-1.750867  , -0.115253696, -1.1425925 , -0.79185915, -0.48000807,
        %.  0.05481249, -0.06936351, -0.17544615,  0.6582494 , -0.7127066 ],
    
    % 8 0.320556640625 7 0.140533447265625 1 0.193817138671875 5 0.067138671875 9 0.107025146484375 3 0.04205322265625 2 0.09515380859375 0 0.030731201171875 4 0.002777099609375 6 0.000213623046875

    \begin{subfigure}[t]{0.115\textwidth}
    \centering
    Frequency
    \end{subfigure}
    
    \begin{subfigure}[t]{0.081\textwidth}
    \centering
    $3.07\%$
    \end{subfigure}
    
    &
    
    \begin{subfigure}[t]{0.081\textwidth}
    \centering
    $19.3\%$
    \end{subfigure}
    
    &
    
    \begin{subfigure}[t]{0.081\textwidth}
    \centering
    $9.51\%$
    \end{subfigure}
    
    &
    
    \begin{subfigure}[t]{0.081\textwidth}
    \centering
    $4.20\%$
    \end{subfigure}
    
    &
    
    \begin{subfigure}[t]{0.081\textwidth}
    \centering
    $0.27\%$
    \end{subfigure}
    
    &
    
    \begin{subfigure}[t]{0.081\textwidth}
    \centering
    $6.71\%$
    \end{subfigure}
    
    &
    
    \begin{subfigure}[t]{0.081\textwidth}
    \centering
    $0.02\%$
    \end{subfigure}
    
    &
    
    \begin{subfigure}[t]{0.081\textwidth}
    \centering
    $14.0\%$
    \end{subfigure}
    
    &
    
    \begin{subfigure}[t]{0.081\textwidth}
    \centering
    $32.0\%$
    \end{subfigure}
    
    &
    
    \begin{subfigure}[t]{0.081\textwidth}
    \centering
    $10.7\%$
    \end{subfigure}
    
    \\
    
            %array([-1.750867  , -0.115253696, -1.1425925 , -0.79185915, -0.48000807,
        %.  0.05481249, -0.06936351, -0.17544615,  0.6582494 , -0.7127066 ],

    % \begin{subfigure}[t]{0.115\textwidth}
    % \centering
    % Weight
    % \end{subfigure}
    
    % \begin{subfigure}[t]{0.081\textwidth}
    % \centering
    % $-1.750$
    % \end{subfigure}
    
    % &
    
    % \begin{subfigure}[t]{0.081\textwidth}
    % \centering
    % $-0.115$
    % \end{subfigure}
    
    % &
    
    % \begin{subfigure}[t]{0.081\textwidth}
    % \centering
    % $-1.142$
    % \end{subfigure}
    
    % &
    
    % \begin{subfigure}[t]{0.081\textwidth}
    % \centering
    % $-0.791$
    % \end{subfigure}
    
    % &
    
    % \begin{subfigure}[t]{0.081\textwidth}
    % \centering
    % $-0.480$
    % \end{subfigure}
    
    % &
    
    % \begin{subfigure}[t]{0.081\textwidth}
    % \centering
    % $+0.054$
    % \end{subfigure}
    
    % &
    
    % \begin{subfigure}[t]{0.081\textwidth}
    % \centering
    % $-0.069$
    % \end{subfigure}
    
    % &
    
    % \begin{subfigure}[t]{0.081\textwidth}
    % \centering
    % $-0.175$
    % \end{subfigure}
    
    % &
    
    % \begin{subfigure}[t]{0.081\textwidth}
    % \centering
    % $+0.658$
    % \end{subfigure}
    
    % &
    
    % \begin{subfigure}[t]{0.081\textwidth}
    % \centering
    % $-0.712$
    % \end{subfigure}

    \end{tabular}
\caption{Random selection of frames from each cluster along with their corresponding relative frequency. 
Clusters \#1, \#7, \#8 are more informative and their contribution is higher than other clusters.}
\label{fig:samples}
\end{figure}{}

\begin{figure*}[h]

\centering
\captionsetup[subfigure]{labelformat=empty,justification=centering,aboveskip=1pt,belowskip=1pt}
    \begin{tabular}[c]{l r}
    \centering
    
    \begin{subfigure}[t]{0.5\textwidth}
        \begin{tikzpicture}
            \begin{axis}[
            enlarge y limits=true,
            width=6.25cm, height=5cm,
            xlabel={$Q_{\text{Offline}}$},
            ylabel={Detection},
            axis lines=left,
            ylabel near ticks,
            xlabel near ticks,
            scaled ticks=true,
            clip=false,
            ]
            \addplot[only marks, color=red, mark=*, mark size=1.2pt] table [x=predict, y=detect, col sep=comma] {figures/global/data/measures-global-10c_5.csv};
            \end{axis}
        
        \end{tikzpicture}

    \end{subfigure}
    
    &
    
    \begin{subfigure}[t]{0.5\textwidth}
        \begin{tikzpicture}
            \begin{axis}[
            enlarge y limits=true,
            width=6.25cm, height=5cm,
            xlabel={$Q_{\text{Offline}}$},
            ylabel={\# Polyps},
            axis lines=left,
            ylabel near ticks,
            xlabel near ticks,
            scaled ticks=true,
            clip=false,
            ]
            \addplot[only marks, color=blue, mark=*, mark size=1.2pt] table [x=predict, y=polyp, col sep=comma] {figures/global/data/measures-global-10c_5.csv};
            \end{axis}
        
        \end{tikzpicture}
    \end{subfigure}
    
    \end{tabular}
\caption{Analyzing the relationship between the suggested method and the absolute polyp frame detection scores (left) and the true number of polyps found in the procedure (right). As can be seen, the proposed measure is strongly correlated with the presence of polyps.}
\label{fig:buckets_and_hists}
\end{figure*}

\begin{table*}[h!]
    \scriptsize
	\begin{center}
		\begin{tabular}{c||c||c}
			Encoder, $f_\theta (\cdot)$ & Projection, $g_{\phi} (\cdot)$ & Classifier\\ \hline \hline
			\begin{tabular}{ c c c }
				c1 & $112\times 112$ & $\begin{bmatrix} 3 \times 3, 64, s2 \\ 3 \times 3, 64 \\ 3 \times 3, 64  \end{bmatrix} \times 1 $ \\
				c2 & $56\times 56$ & $\begin{bmatrix} 1 \times 1, 64 \\ 3 \times 3, 64 \\ 1 \times 1, 256  \end{bmatrix} \times 3 $ \\
				c3 & $28\times 28$ & $\begin{bmatrix} 1 \times 1, 128 \\ 3 \times 3, 128 \\ 1 \times 1, 512  \end{bmatrix} \times 4 $ \\
				c4 & $14\times 14$ & $\begin{bmatrix} 1 \times 1, 256 \\ 3 \times 3, 256 \\ 1 \times 1, 1024  \end{bmatrix} \times 23 $ \\
				c5 & $7\times 7$ & $\begin{bmatrix} 1 \times 1, 512 \\ 3 \times 3, 512 \\ 1 \times 1, 2048  \end{bmatrix} \times 3 $
			\end{tabular} 
			
			& 
			
			\begin{tabular}{ c c c }
				head & $1\times 1$ & $\begin{bmatrix} \text{Avg pool}\\ \text{Dropout}\\ \text{FC}, 512  \end{bmatrix} \times 1 $
				
			\end{tabular}
			
			& 
			
			\begin{tabular}{ c c c }
				Classifier & $1\times 1$ & $\begin{bmatrix} \text{FC}, 10 \\ \text{Sigmoid}  \end{bmatrix} \times 1 $
				
			\end{tabular}
		\end{tabular}
		\caption{We use ResNet-RS50 for the encoder and a simple MLP with one hidden layer for the projection head, as suggested in SIMCLR. Additionally, for the classifier, we use a single linear layer. The frame encoder model is trained for $100k$ training steps with a batch-size of $512$. Whereas, the classifier is trained for $500$ epochs with a batch-size of $64$. For both training schemes, we use the Adam optimizer with a piecewise constant learning rate decay.}
	\end{center}
\end{table*}

% \bibliographystyle{splncs04}
% \bibliography{references}
\end{document}
