# Supplementary material for: Semi-supervised Quality Evaluation of Colonoscopy Procedures
Source: arXiv:2305.10090 source file (2023-05-17)
Supplement: Supplementary file 2 [file sm.tex]

\begin{figure}
\centering
\captionsetup[subfigure]{labelformat=empty,justification=centering,aboveskip=1pt,belowskip=1pt}
    \begin{tabular}[c]{c c c c c c c c c c c}
    
    \centering
    
    \begin{subfigure}[t]{0.115\textwidth}
    \centering
    \caption*{Cluster}
    \end{subfigure}
    
    \begin{subfigure}[t]{0.081\textwidth}
    \centering
    \caption*{\#0}
    \end{subfigure}
    
    &
    
    \begin{subfigure}[t]{0.081\textwidth}
    \centering
    \caption*{\#1}
    \end{subfigure}
    
    &
    
    \begin{subfigure}[t]{0.081\textwidth}
    \centering
    \caption*{\#2}
    \end{subfigure}
    
    &
    
    \begin{subfigure}[t]{0.081\textwidth}
    \centering
    \caption*{\#3}
    \end{subfigure}
    
    &
    
    \begin{subfigure}[t]{0.081\textwidth}
    \centering
    \caption*{\#4}
    \end{subfigure}
    
    &
    
    \begin{subfigure}[t]{0.081\textwidth}
    \centering
    \caption*{\#5}
    \end{subfigure}
    
    &
    
    \begin{subfigure}[t]{0.081\textwidth}
    \centering
    \caption*{\#6}
    \end{subfigure}
    
    &
    
    \begin{subfigure}[t]{0.081\textwidth}
    \centering
    \caption*{\#7}
    \end{subfigure}
    
    &
    
    \begin{subfigure}[t]{0.081\textwidth}
    \centering
    \caption*{\#8}
    \end{subfigure}
    
    &
    
    \begin{subfigure}[t]{0.081\textwidth}
    \centering
    \caption*{\#9}
    \end{subfigure}
    
    \\

    \begin{subfigure}[t]{0.115\textwidth}
    \centering
    \vspace{1.9cm}
    Samples
    \end{subfigure}
    
    \begin{subfigure}[t]{0.081\textwidth}
    \centering
    \includegraphics[width=1\linewidth]{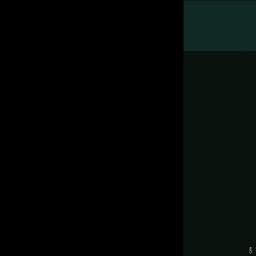}
    \includegraphics[width=1\linewidth]{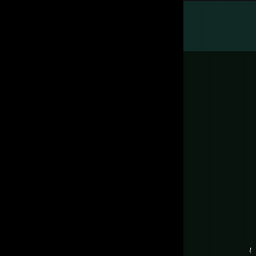}
    \includegraphics[width=1\linewidth]{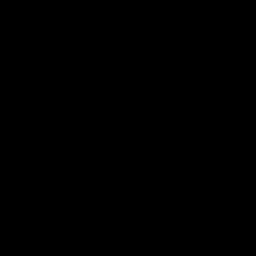}
    \includegraphics[width=1\linewidth]{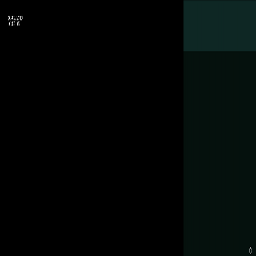}
    \includegraphics[width=1\linewidth]{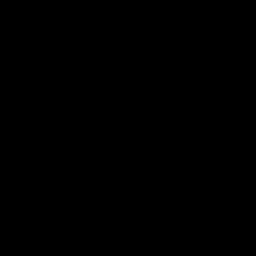}
    \includegraphics[width=1\linewidth]{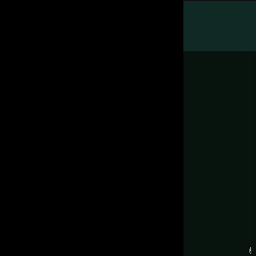}
    \end{subfigure}
    
    &
    
    \begin{subfigure}[t]{0.081\textwidth}
    \centering
    \includegraphics[width=1\linewidth]{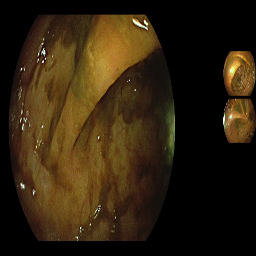}
    \includegraphics[width=1\linewidth]{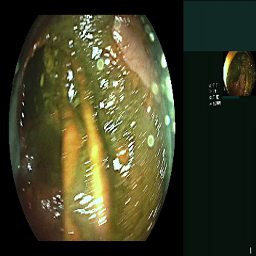}
    \includegraphics[width=1\linewidth]{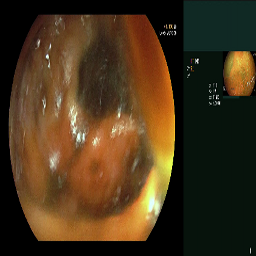}
    \includegraphics[width=1\linewidth]{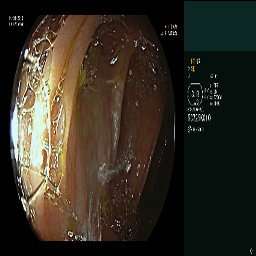}
    \includegraphics[width=1\linewidth]{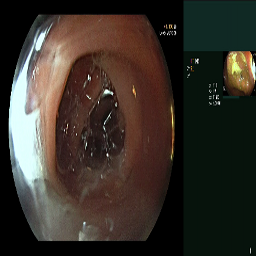}
    \includegraphics[width=1\linewidth]{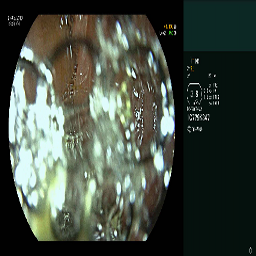}
    \end{subfigure}
    
    &
    
    \begin{subfigure}[t]{0.081\textwidth}
    \centering
    \includegraphics[width=1\linewidth]{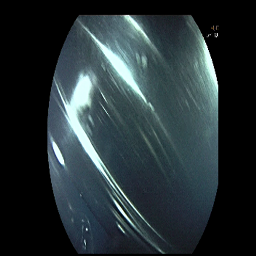}
    \includegraphics[width=1\linewidth]{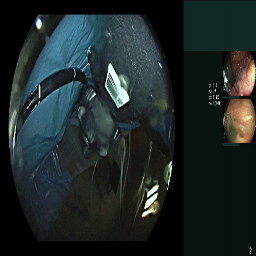}
    \includegraphics[width=1\linewidth]{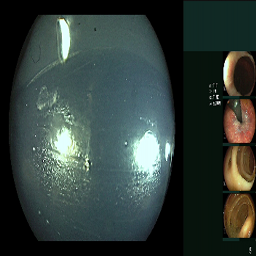}
    \includegraphics[width=1\linewidth]{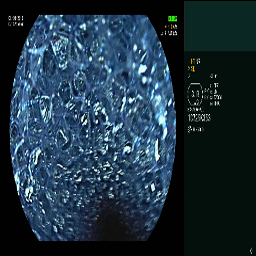}
    \includegraphics[width=1\linewidth]{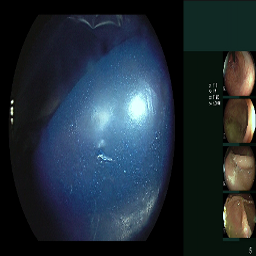}
    \includegraphics[width=1\linewidth]{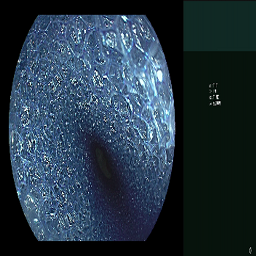}
    \end{subfigure}
    
    &
    
    \begin{subfigure}[t]{0.081\textwidth}
    \centering
    \includegraphics[width=1\linewidth]{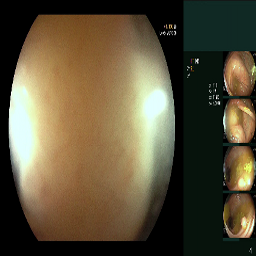}
    \includegraphics[width=1\linewidth]{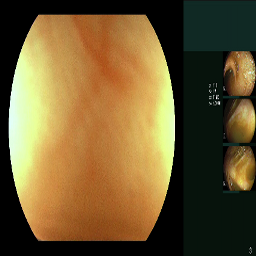}
    \includegraphics[width=1\linewidth]{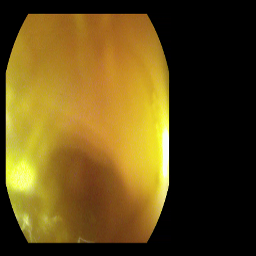}
    \includegraphics[width=1\linewidth]{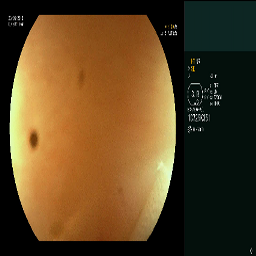}
    \includegraphics[width=1\linewidth]{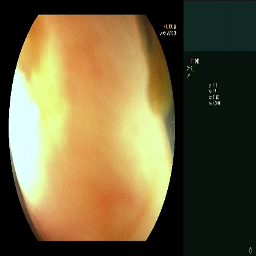}
    \includegraphics[width=1\linewidth]{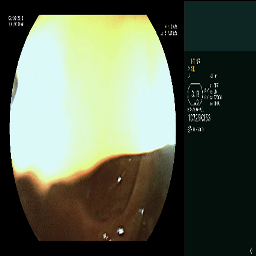}
    \end{subfigure}
    
    &
    
    \begin{subfigure}[t]{0.081\textwidth}
    \centering
    \includegraphics[width=1\linewidth]{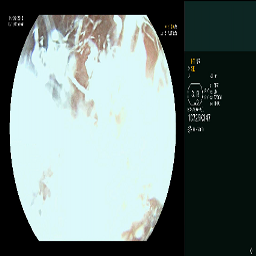}
    \includegraphics[width=1\linewidth]{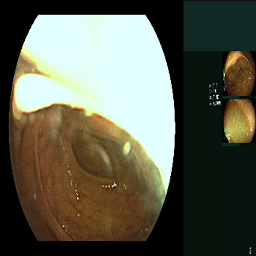}
    \includegraphics[width=1\linewidth]{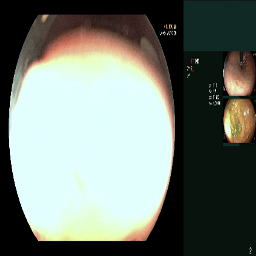}
    \includegraphics[width=1\linewidth]{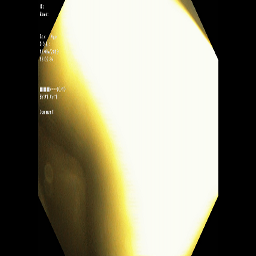}
    \includegraphics[width=1\linewidth]{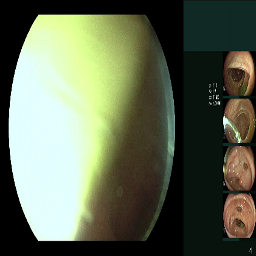}
    \includegraphics[width=1\linewidth]{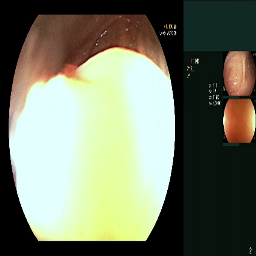}
    
    \end{subfigure}
    
    &
    
    \begin{subfigure}[t]{0.081\textwidth}
    \centering
    \includegraphics[width=1\linewidth]{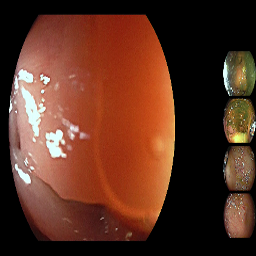}
    \includegraphics[width=1\linewidth]{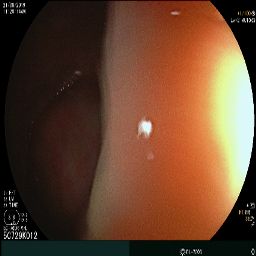}
    \includegraphics[width=1\linewidth]{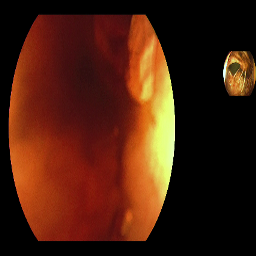}
    \includegraphics[width=1\linewidth]{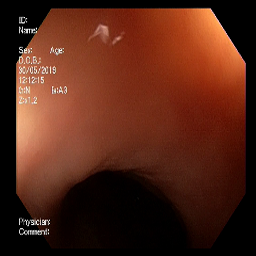}
    \includegraphics[width=1\linewidth]{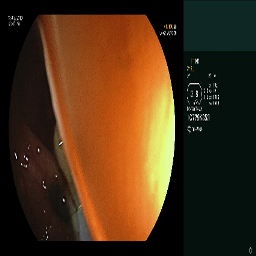}
    \includegraphics[width=1\linewidth]{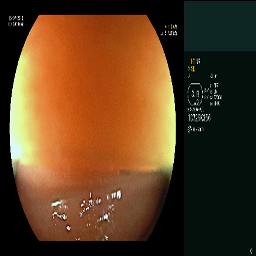}
    \end{subfigure}
    
    &
    
    \begin{subfigure}[t]{0.081\textwidth}
    \centering
    \includegraphics[width=1\linewidth]{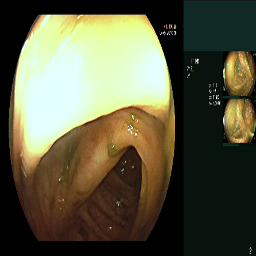}
    \includegraphics[width=1\linewidth]{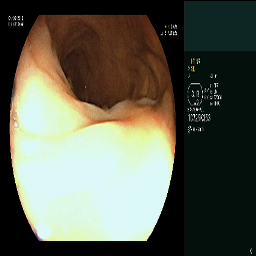}
    \includegraphics[width=1\linewidth]{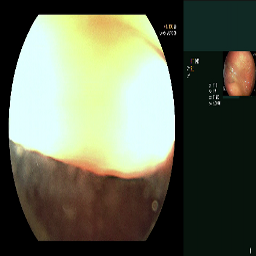}
    \includegraphics[width=1\linewidth]{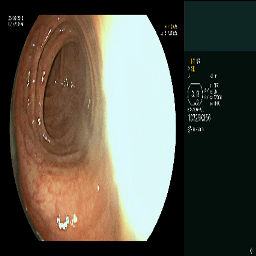}
    \includegraphics[width=1\linewidth]{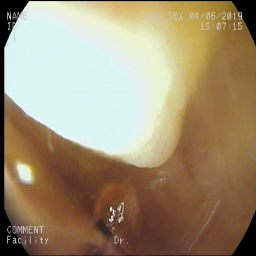}
    \includegraphics[width=1\linewidth]{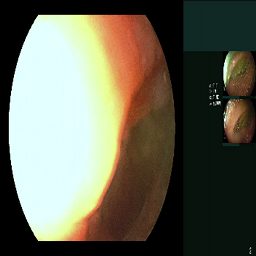}
    \end{subfigure}
    
    &
    
    \begin{subfigure}[t]{0.081\textwidth}
    \centering
    \includegraphics[width=1\linewidth]{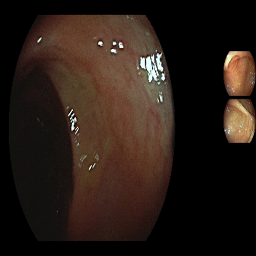}
    \includegraphics[width=1\linewidth]{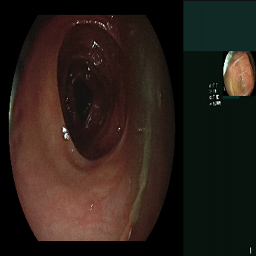}
    \includegraphics[width=1\linewidth]{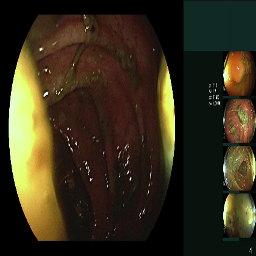}
    \includegraphics[width=1\linewidth]{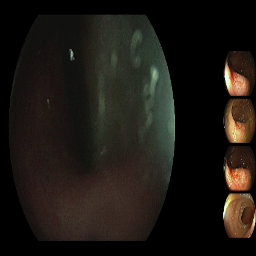}
    \includegraphics[width=1\linewidth]{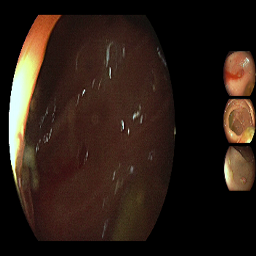}
    \includegraphics[width=1\linewidth]{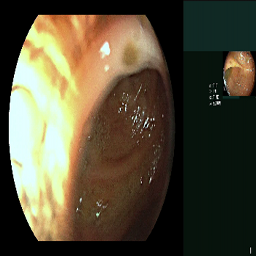}
    \end{subfigure}
    
    &
    
    \begin{subfigure}[t]{0.081\textwidth}
    \centering
    \includegraphics[width=1\linewidth]{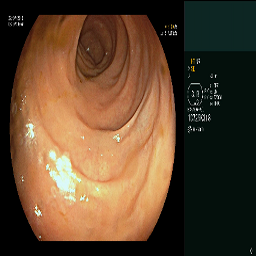}
    \includegraphics[width=1\linewidth]{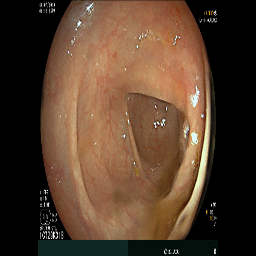}
    \includegraphics[width=1\linewidth]{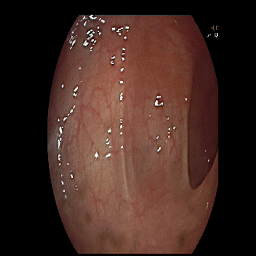}
    \includegraphics[width=1\linewidth]{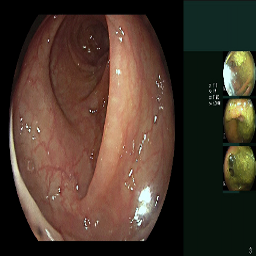}
    \includegraphics[width=1\linewidth]{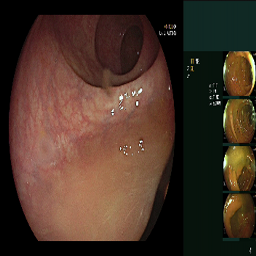}
    \includegraphics[width=1\linewidth]{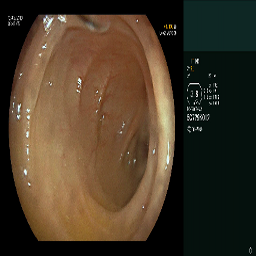}
    \end{subfigure}
    
    &
    
    \begin{subfigure}[t]{0.081\textwidth}
    \centering
    \includegraphics[width=1\linewidth]{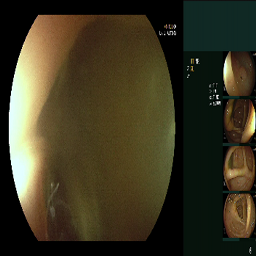}
    \includegraphics[width=1\linewidth]{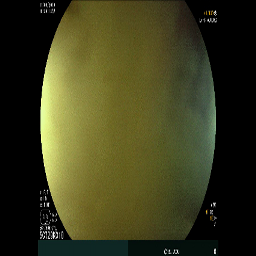}
    \includegraphics[width=1\linewidth]{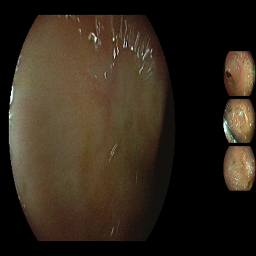}
    \includegraphics[width=1\linewidth]{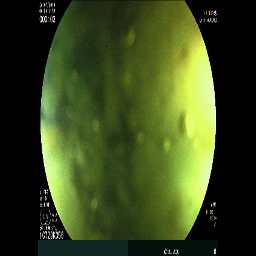}
    \includegraphics[width=1\linewidth]{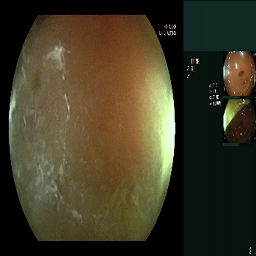}
    \includegraphics[width=1\linewidth]{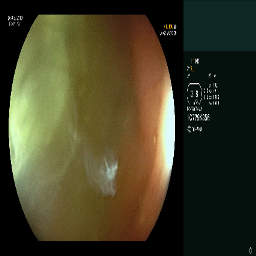}
    \end{subfigure}
    
    \\
        %array([-1.750867  , -0.115253696, -1.1425925 , -0.79185915, -0.48000807,
        %.  0.05481249, -0.06936351, -0.17544615,  0.6582494 , -0.7127066 ],
    
    % 8 0.320556640625 7 0.140533447265625 1 0.193817138671875 5 0.067138671875 9 0.107025146484375 3 0.04205322265625 2 0.09515380859375 0 0.030731201171875 4 0.002777099609375 6 0.000213623046875

    \begin{subfigure}[t]{0.115\textwidth}
    \centering
    Frequency
    \end{subfigure}
    
    \begin{subfigure}[t]{0.081\textwidth}
    \centering
    $3.07\%$
    \end{subfigure}
    
    &
    
    \begin{subfigure}[t]{0.081\textwidth}
    \centering
    $19.3\%$
    \end{subfigure}
    
    &
    
    \begin{subfigure}[t]{0.081\textwidth}
    \centering
    $9.51\%$
    \end{subfigure}
    
    &
    
    \begin{subfigure}[t]{0.081\textwidth}
    \centering
    $4.20\%$
    \end{subfigure}
    
    &
    
    \begin{subfigure}[t]{0.081\textwidth}
    \centering
    $0.27\%$
    \end{subfigure}
    
    &
    
    \begin{subfigure}[t]{0.081\textwidth}
    \centering
    $6.71\%$
    \end{subfigure}
    
    &
    
    \begin{subfigure}[t]{0.081\textwidth}
    \centering
    $0.02\%$
    \end{subfigure}
    
    &
    
    \begin{subfigure}[t]{0.081\textwidth}
    \centering
    $14.0\%$
    \end{subfigure}
    
    &
    
    \begin{subfigure}[t]{0.081\textwidth}
    \centering
    $32.0\%$
    \end{subfigure}
    
    &
    
    \begin{subfigure}[t]{0.081\textwidth}
    \centering
    $10.7\%$
    \end{subfigure}
    
    \\
    
            %array([-1.750867  , -0.115253696, -1.1425925 , -0.79185915, -0.48000807,
        %.  0.05481249, -0.06936351, -0.17544615,  0.6582494 , -0.7127066 ],

    % \begin{subfigure}[t]{0.115\textwidth}
    % \centering
    % Weight
    % \end{subfigure}
    
    % \begin{subfigure}[t]{0.081\textwidth}
    % \centering
    % $-1.750$
    % \end{subfigure}
    
    % &
    
    % \begin{subfigure}[t]{0.081\textwidth}
    % \centering
    % $-0.115$
    % \end{subfigure}
    
    % &
    
    % \begin{subfigure}[t]{0.081\textwidth}
    % \centering
    % $-1.142$
    % \end{subfigure}
    
    % &
    
    % \begin{subfigure}[t]{0.081\textwidth}
    % \centering
    % $-0.791$
    % \end{subfigure}
    
    % &
    
    % \begin{subfigure}[t]{0.081\textwidth}
    % \centering
    % $-0.480$
    % \end{subfigure}
    
    % &
    
    % \begin{subfigure}[t]{0.081\textwidth}
    % \centering
    % $+0.054$
    % \end{subfigure}
    
    % &
    
    % \begin{subfigure}[t]{0.081\textwidth}
    % \centering
    % $-0.069$
    % \end{subfigure}
    
    % &
    
    % \begin{subfigure}[t]{0.081\textwidth}
    % \centering
    % $-0.175$
    % \end{subfigure}
    
    % &
    
    % \begin{subfigure}[t]{0.081\textwidth}
    % \centering
    % $+0.658$
    % \end{subfigure}
    
    % &
    
    % \begin{subfigure}[t]{0.081\textwidth}
    % \centering
    % $-0.712$
    % \end{subfigure}

    \end{tabular}
\caption{Random selection of frames from each cluster along with their corresponding relative frequency. 
Clusters \#1, \#7, \#8 are more informative and their contribution is higher than other clusters.}
\label{fig:samples}
\end{figure}{}
